# Supplementary material for: BankTweak: Adversarial Attack against Multi-Object Trackers by Manipulating Feature Banks
Source: arXiv:2408.12727 source file (2024-08-22)
Supplement: Supplementary file 1 [file 06appendix.tex]

\section{Appendix}
